# Supplementary material for: Deuce: A Lightweight User Interface for Structured Editing
Source: arXiv:1707.00015 source file (2018-02-05)
Supplement: Supplementary file 1 [file appendix-discussion.tex]

\section{Additional Discussion}

The primary motivation for
our work is to demonstrate how a variety of structured
transformations---not just refactorings---can be supported with
automated tooling in a lightweight, text-editing workflow
(\cf{}~\autoref{sec:intro}). Our approach also aims to
simplify the steps to identify, invoke, and configure
transformations provided by refactoring tools
(\cf{}~\autoref{sec:discussion-related-dndr}).

\citet{FlossRefactoring} define five desired characteristics that a
\emph{floss refactoring} tool ought to satisfy. We refine these
criteria below according to our motivation, with changes marked in bold.
Compared to the original
criteria, we generalize the goals of such tools slightly in order to
(a) support transformations beyond refactorings, and (b) provide a seamless
interface for interacting with the user in situations where
configuration cannot be avoided (\eg{} to make choices about variable
names and function boundaries).

%% Because our motivation is to design a user interface that allows a
%% variety of structured transformations---not just refactorings---to be
%% supported with automated tooling in a lightweight, text-editing workflow,
%% we refine these criteria below, with changes marked in bold.

\begin{enumerate}
\item Choose the desired \textbf{structured transformation} quickly,
\item Switch seamlessly between program editing and
\textbf{structured transformations},
\item View and navigate the program code while using the tool,
\item Avoid providing explicit configuration information,
\textbf{but do so seamlessly when needed}, and
\item Access all the other
tools normally available in the
development environment while using the \textbf{structured editing}
tool.
\end{enumerate}

\noindent
We believe \deuce{} represents a proof-of-concept for how to achieve
these goals for ``floss structured editing.''
We hope that our ideas will help inform future progress on making
refactoring and structured editing a more common part of a typical
programming workflow.

\subsection{Related Work --- Refactorings and Other Transformations}

\parahead{Refactoring for Functional Languages}

\hare{}~\cite{Thompson2013,HaReThesis1,HaReThesis2}
provides many transformations that are common when programming in
functional languages, such as Haskell,
where features including first-class functions
(\ie{} lambdas), local bindings, tuples, algebraic datatypes, and type
polymorphism lead to tasks---such as Promote to Outer Scope, Demote to
Inner Scope, and Generalize Expression---that are more
``fine-grained'' tasks than those supported in most typical
refactoring tools for object-oriented programs. Like refactoring tools
for object-oriented languages, \hare{} employs a menu-based user
interface (implemented in Emacs and Vim), which requires one of the named
transformations to be explicitly selected from a menu
%% (\rkc{with the mouse or keyboard hotkeys})
and applied to the desired expressions in the code.
Our user interface could be incorporated by \hare{} to expose the
supported transformations with lightweight, direct manipulation
features.

%% Our user interface in \deuce{} is intended to be a lightweight, direct
%% manipulation interface for invoking such transformations.

\hare{} provides a large catalog of transformations, many more than in
our current implementation of \deuce{}. However, some of our
transformations are, to the best of our knowledge, not found in
existing tools. For example, \hare{} provides Promote and Demote
transformations for moving definitions into adjacent (outer and inner,
respectively) expressions, whereas our Move Definition tools allow
reordering of non-adjacent definitions, as well as dependency inversion.
Also, the Make Equal tool is a non-semantics preserving transformation
that we have found useful during the prototyping and repair phases of
development. Lastly, we have implemented some domain-specific
transformations useful in the setting of functional programming to
generate SVGs.

\parahead{Transformations for Program Development}

\citet{Reichenbach:2009}
identify the role of \emph{program metamorphosis}, where intermediate
steps of a transformation do not preserve behavior, or even
where the overall transformation is intended to selectively deviate
from the original. \citet{Steimann:2012} describe a tool for
supporting refactorings that are specifically tailored to the
particular program and task at hand and, thus, do not have
well-established names.
A goal of our work is to promote automated support for structured
transformations throughout all phases of development, including ones
which change program behavior and which may even be tailored to a
specific domain or program.

While the majority of work on structured editors has focused on user
interfaces and tools, relatively little has been developed about the
meanings of programs that are undergoing transformations.
\citet{HazelnutPOPL} define a calculus
that serves as a foundation for reasoning about edits to an AST. A
particularly interesting aspect of their work is their account for
incomplete programs where \emph{holes} have yet to be filled in. The
programming process consists of iteratively transforming an incomplete
program into a final one, so these foundations may help to inform the
goals and design for the kinds of interactive editing environments
that \deuce{} and many other structured editing tools aim to provide.

\subsection{Future Work}

We see several directions for subsequent work. One is to adapt and
implement our approach for existing, full-featured programming
languages and existing development environments. Another is to
incorporate additional well-known transformations
(\eg{}~\cite{Fowler1999,Thompson2013}). Independent of these choices
about target language and transformations, there are several
opportunities to improve on our methodology.

\parahead{User Interface}

There are several opportunities to improve the user interface for invoking
transformations.

%% With respect to the selection of structural features, it would be
%% useful to have a more sophisticated presentation than our bounding
%% polygons, so that it is easier to select components among deeply
%% nested structures. Furthermore, it would be useful to denote target
%% positions by a more expansive notion of space between expressions
%% rather than using only the single characters before and after items.

\paragraph{Direct Manipulation Gestures}
While our approach supports invoking transformations
that require multiple selections, it would be useful to support
drag-and-drop gestures (as in \dndr{}) for the subset of transformations
that require a single source item and single target expression.
For transformations that do not fit in the single-source single-target
paradigm, it would be useful to perform user studies, following the
approach of \citet{DNDRefactoring}, to identify intuitive mappings for more
specific direct manipulation gestures than the selection- and
menu-based approach in \deuce{}. For example, to invoke the Make
Equal tool to copy expressions, two alternative user actions could
be to (i) treat the first selection as the one to copy to the rest or
(ii) select all of the expressions to be modified and then drag the
expression to copy to one of them (which would copy the expression to
all selections).

It would also be useful to provide information about selected
widgets that are offscreen; these are currently not shown.
Alternatives include information at the borders of the code editor to
summarize the selection state of items in each direction, and a
scrolling side bar view that depicts the entire program and relevant
areas of selection state.

\paragraph{Code Diffs}
To help explain each of the suggested transformations, our visual previews may
be augmented to show code diffs, instead of just the transformed code as in
our current implementation.  It may also help to draw additional
information on the source code relevant to a transformation---for
example, arrows between source and target expressions, and between
variable uses and definitions (as in
DrRacket~(\url{https://racket-lang.org/}))---and to smoothly
animate the code edits to further help explain the automated
transformations.

\paragraph{Discoverability}
While our current approach displays which transformations are active
given the selection state, it could further help discoverability to
show what transformations may be active if additional items are
selected. The challenge here is to display suggestions for selections
and transformations that may be of interest without cluttering the
display and overwhelming the user with too many choices.

\parahead{Domain-Specific Language for Transformations}

If a \little{} transformation can be implemented in terms of the
active selections of a program, it can easily be plugged into our
menu-based approach. To make the approach even more extensible, it would be
useful to design a domain-specific language of rewrite rules and
appropriate side conditions, so that
\deuce{} may be instantiated with different transformations in
different settings without having to implement each inside the tool.

\parahead{Adaptive Concrete Syntax}

Our approach embraces plain text as a desirable format for programs,
and, thus, the importance for programmers to make judicious choices about
variable names, whitespace, and other formatting properties. Tools
such as Move Definitions, Align Expressions, and Make Multi-Line
provide a modicum of
help when making these decisions, but there are still many factors
that the user must consider entirely on her own---such as
screen sizes, style
conventions, changes in expressions that make them shorter or longer.

It may be interesting to consider how the editor could automatically
convert between different plain text formats as these different
criteria change. For example, maybe a particular multi-way definition
is a good choice when, say, the maximum suggested line width for a
given project is 80 characters but not when it is 60 characters. In
addition to the transformations currently implemented in \deuce{} that
help the user perform transformations on the \emph{abstract} syntax of
the program, transformations could help manipulate the \emph{concrete}
syntax as well.
%% Our implementation currently includes a monolithic Clean Up tool that
%% runs a collection of rewrite rules, including ones that insert and
%% remove whitespace and line breaks, on the entire program. Selectively
%% applying such rules to selected expressions could help the user arrive
%% at the final formatting and structure of the code.

%% concrete syntax is irrelevant, hence structured editing
%% 
%% but test is unavoidable, and concrete syntax and style is important
%% 
%% for example, one common use of move defs is to make things fit nicely, but this
%% depends on screen sizes, style conventions, changes to the expressions
%% 
%% auto-reformat

\parahead{Incremental, Structure-Aware Parsing}

Toggling between text- and mouse-based editing in \deuce{} is achieved
with a quick keystroke, but the complete separation between modes has limitations.
As soon there are any character changes to the text, the structure
information (and any active transformations) become invalidated. It
would be better to incorporate an incremental
parsing approach~(\eg{}~\cite{Wagner:1998} as used by
Barista~\citep{Barista}) to tolerate some degree of
differences in the source text, so that as much of the structure
information as possible can persist even while the code
has been changed with text-edits. This would help to further
streamline, and augment, the support for structured editing within the
full, unrestricted text-editing workflow.
